# Supplementary material for: Zero-Sum Stochastic Stackelberg Games
Source: arXiv:2211.13847 source file (2022-11-25)
Supplement: Supplementary file 2 [file appendix.tex]

% \section{Ommited Results and Proofs \Cref{sec:prelim}}\label{sec_app:prelim}



% \if 0
% We now move on to investigate the existence properties of Stackelberg equilibria. To this end, we first define the following operators: $\statevalue[][][][\actionvalfuncs \times \outerset^\states \times \innerset^\states]: \actionvalfuncs \times \outerset^\states \times \innerset^\states \to \statevalfuncs$, $\actionvalue[][][][\statevalfuncs \times \outerset^\states \times \innerset^\states]: \statevalfuncs \times \outerset^\states \times \innerset^\states \to \actionvalfuncs$, and $\argval[\actionvalfuncs] : \actionvalfuncs \to \outerset^\states \times \innerset^\states$: 
% \begin{align}
%     \left(\statevalue[][][][\actionvalfuncs \times \outerset^\states \times \innerset^\states](\actionvalue, \policy[\outer], \policy[\inner])\right)(\state) = \actionvalue(\state, \policy[\outer](\state), \policy[\inner](\state))\label{eq:v_operator}
% \end{align}

% \begin{align}
%     \left(\actionvalue[][][][\statevalfuncs \times \outerset^\states \times \innerset^\states](\statevalue, \policy[\outer], \policy[\inner])\right)(\state, \outer, \inner) = \mathop{\E}_{\staterv^\prime \sim \trans(\cdot \mid \state, \outer, \inner)} \left[ \reward(\state, \outer, \inner) + \discount \statevalue(\staterv^\prime) \right]\label{eq:q_operator}
% \end{align}

% \begin{align}
%     \argval[\actionvalfuncs](\actionvalue) = \left\{(\policy[\outer]^*, \policy[\inner]^*) 
%     % \in \outerset^\states \times \innerset^\states
%     \mid  \forall \state,  \max_{\inner \in \innerset : \constr(\state, \policy[\outer]^*(\state), \inner) \geq \zeros}  \actionvalue[][{\policy[\outer]^*} ][{\policy[\inner]^*}](\state, \policy[\outer]^*(\state), \inner) \leq \statevalue[][{\policy[\outer]^*}][ {\policy[\inner]^*}](\state)  \leq \min_{\outer \in \outerset} \max_{\inner \in \innerset : \constr(\state, \outer, \inner) \geq \zeros} \actionvalue[][{\policy[\outer]^*}][ {\policy[\inner]^*}](\state, \outer, \inner)\right\}
% \end{align}


% \begin{theorem}
% Given a stochastic min-max Stackelberg game $(\states, \outerset, \innerset, \initstates, \reward, \constr, \trans, \discount)$, if there exists $\actionvalue \in \actionvalfuncs$, $\policy[\outer] \in \outerset^\states$, and $\policy[\inner] \in \innerset^\states$ such that
% %
% $\statevalue = \statevalue[][][][\actionvalfuncs \times \outerset^\states \times \innerset^\states](\actionvalue, \policy[\outer], \policy[\inner])$, 
% %
% $\actionvalue = \actionvalue[][][][\statevalfuncs \times \outerset^\states \times \innerset^\states](\statevalue, \policy[\outer], \policy[\inner])$,
% %
% and
% $(\policy[\outer],  \policy[\inner]) \in \argval[\actionvalfuncs](\actionvalue)$, then $(\policy[\outer]^*, \policy[\inner]^*)$ is a Stackelberg equilibrium of $(\states, \outerset, \innerset, \initstates, \reward, \constr, \trans, \discount)$ and we have
% $\statevalue = \statevalue[][{\policy[\outer]}][{\policy[\inner]}]$, $\actionvalue = \actionvalue[][{\policy[\outer]}][{\policy[\inner]}]$.
% %  
% \end{theorem}

% \begin{proof}
% By \Crefrange{eq:v_operator}{eq:q_operator} we have for all states $\state \in \states$:
% \begin{align}
%     &\statevalue[](\state) = \actionvalue[](\state, \policy[\outer](\state), \policy[\inner](\state))\\
%     &\actionvalue[](\state, \outer, \inner) = \mathop{\E}_{\staterv^\prime \sim \trans(\cdot \mid \state, \outer, \inner)} \left[ \reward(\state, \outer, \inner) +  \discount \statevalue[](\staterv^\prime)  \right]
% \end{align}
% Therefore, by \Cref{thm:bellman}, we have that $\statevalue = \statevalue[][{\policy[\outer]}][{\policy[\inner]}]$, $\actionvalue = \actionvalue[][{\policy[\outer]}][{\policy[\inner]}]$. Additionally, by 
%  \Cref{thm:equiv_def_stackelberg} and the definition of $\argval[\actionvalfuncs](\actionvalue)$, we know that $(\policy[\outer],  \policy[\inner])$ is a Stackelberg equilibrium.
% \end{proof}

% Using the above, we construct a function $\policyfp: \actionvalfuncs \times \outerset^\states \times \innerset^\states \to  \actionvalfuncs \times \outerset^\states \times \innerset^\states$ such that $\policyfp = \left(I \times \argval[\actionvalfuncs]\right) \circ \actionvalue[][][][\statevalfuncs \times \outerset^\states \times \innerset^\states] \circ \statevalue[][][][\actionvalfuncs \times \outerset^\states \times \innerset^\states]$ where $I$ is the identity operator. The following corollary of \Cref{thm:bellman} applies to to $\policyfp$:

% \begin{corollary}\label{corr:fp_stackelberg}
% Given a stochastic min-max Stackelberg game $(\states, \outerset, \innerset, \initstates, \reward, \constr, \trans, \discount)$, if there exists a fixed point $(\actionvalue, \policy[\outer], \policy[\inner])$ such that $(\actionvalue, \policy[\outer], \policy[\inner]) \in \policyfp(\actionvalue, \policy[\outer], \policy[\inner])$, then $(\policy[\outer], \policy[\inner])$ is a Stackelberg equilibrium, and $\actionvalue = \actionvalue[][{\policy[\outer]}][{\policy[\inner]}]$.
% \end{corollary}



% \begin{lemma}
% The set of Stackelberg equilibria of any min-max Stackelberg game $(\outerset, \innerset, \obj, \constr)$ is non-empty, compact, and convex.
% \end{lemma}
% \begin{proof}
% By proposition B.2 from \cite{goktas2021minmax}, the set of Stackelberg equilibria of any min-max Stackelberg game is non-empty. Additionally, under \Cref{assum:main}, we have that for all $\outer \in \outers$, $\obj(\outer, \cdot)$ is concave, and $\{\inner \innerset \mid \constr(\outer, \inner) \geq \zeros\}$ is convex. Hence, by \cite{} the set of solutions $\outerset^*(\outer) = \argmax_{\inner \in \innerset: \constr(\outer, \inner) \geq \zeros} \obj(\outer, \inner)$ is compact- and convex- valued.
% %
% Similarly, under \Cref{assum:main}, by proposition B.1 from \cite{goktas2021minmax}, $\max_{\inner \in \innerset: \constr(\outer, \inner) \geq \zeros} \obj(\outer, \inner)$ is continuous and convex. Hence, the set of solutions $\innerset^* = \argmin_{\outer \in \outerset} \max_{\inner \in \innerset: \constr(\outer, \inner) \geq \zeros} \obj(\outer, \inner)$ is compact- and convex-valued. Since the carthesian product of two compact-convex-valued correspondences is compact-convex-valued, we have that the set of Stackelberg equilbiria $\outerset^*\left(\innerset^*\right)$ is also compact-convex-valued.
% \end{proof}

% \begin{corollary}
% The correspondence $\argval[\actionvalfuncs]$ is non-empty-, compact-, convex-valued.
% \end{corollary}

% \begin{proof}
% For any $\actionvalue \in \actionvalfuncs$ and for all states $\state \in \states$, we have that $\left( \argval[\actionvalfuncs](\actionvalue) \right)(\state)$ is the set of Stackelberg equilibria of the min-max Stackelberg game $(\outerset, \innerset, \actionvalfuncs, \constr(\state, \cdot, \cdot))$ which is non-empty-compact-convex-valued. Hence, $\argval[\actionvalfuncs](\actionvalue)$ must be non-empty-compact-convex valued as well since it is the product of multiple non-empty-compact-convex sets.
% \end{proof}

% \begin{lemma}\label{lemma:fp_existence}
% The correspondence $\policyfp$ has a fixed point $(\actionvalue, \policy[\outer], \policy[\inner])$ such that $(\actionvalue, \policy[\outer], \policy[\inner]) \in \policyfp(\actionvalue, \policy[\outer], \policy[\inner])$.
% \end{lemma}
% \begin{proof}
% $\policyfp: \actionvalfuncs \times \outerset^\states \times \innerset^\states \to \actionvalfuncs \times \outerset^\states \times \innerset^\states$ is non-empty-, and convex-valued. It is also compact-valued, i.e., its graph is closed. Hence, by Kakutani's fixed point a fixed point $(\actionvalue, \policy[\outer], \policy[\inner])$ such that $(\actionvalue, \policy[\outer], \policy[\inner]) \in \policyfp(\actionvalue, \policy[\outer], \policy[\inner])$ exists.
% \end{proof}

% \amy{Deni's conjecture: we don't need to assume boundedness in zero-sum games, only in non-zero-sum games}

% Combining \Cref{lemma:fp_existence} and \Cref{corr:fp_stackelberg}, we obtain:
% \begin{theorem}\label{thm:stackelberg_existence}
% Any stochastic min-max Stackelberg game $(\states, \outerset, \innerset, \initstates, \reward, \constr, \trans, \discount)$ has at least one Stackelberg equilibrium 
% \end{theorem}


% \fi
